# Supplementary material for: Navigating the Pitfalls of Active Learning Evaluation: A Systematic Framework for Meaningful Performance Assessment
Source: arXiv:2301.10625 source file (2023-11-03)
Supplement: Supplementary file 1 [file 10_appendix.tex]

\section{Datasets}
% All information is in appendix -> Dataset Description: https://docs.google.com/document/d/1O5b6zTE07QMIIuMsvP2ET0MvFj6nLppfpOMmkTzPt-Q/edit#heading=h.iuu9am48258e 
% TODO: Make this multi column with #valdiation: {#random, #balanced, #validation}, #training, {...}
Each dataset is split into a training \& pool set, a validation set and a test set.\\
For CIFAR-10/100 (LT) datasets the test split of size 10,000 observations is already given and for MIO-TCD and ISIC-2019 we use a custom test split of 25\% random observations of the entire dataset size. 
For MIO-TCD and ISIC-2019 all datasets train, validation and test set are imalanced.\\
The validation sets for all CIFAR-X datasets are 5,000 randomly drawn observations corresponding to 10\% of the entire dataset.
For CIFAR-10 LT the validation dataset is also 5,000 samples big and split of from the dataset before the long-tail distribution is applied onto the training set. The CIFAR-10 LT validation dataset is therefore balanced. 
For MIO-TCD and ISIC-2019 the validation splits consist of 15\% of the entire dataset.\\
The shared training \& pool dataset for CIFAR-10/100 consist of 45,000 observations.
For CIFAR-10 LT the training \& pool datasets consists of ~12,600 observations.
For MIO-TCD and ISIC-2019 the training \& pool datasets consist of 60\% the dataset.
\\
\\
\subsection{Dataset Descriptions}
\paragraph{CIFAR-10} 10 classes, label distribution is uniform
\paragraph{CIFAR-100} 100 classes,label distribution is unfiorm
\paragraph{CIFAR-10 LT} 10 classes, label distribution of train \& pool set is imbalanced, otherwise everything identical to CIFAR-10.\\
The distribution of train \& pool set follows approximately:\\
Class 1: 4500, Class 2: 2913, Class 3: 1886, Class 4: 1221, Class 5: 790, Class 6: 512, Class 7: 331, Class 8: 214, Class 9: 139, Class 10: 90
\paragraph{ISIC-2019} 8 classes, label distribution of the entire dataset is imbalanced.
\\
Class Distribution of entire dataset:
\begin{table}
    \centering
    \begin{tabular}{ll} 
        \toprule
        Class                  & Whole Dataset  \\
        \midrule
        Melanoma               & 4522           \\
        Melanocytic nevus      & 12875          \\
        Basal cell carcinoma   & 3323           \\
        Benign keratosis       & 867            \\
        Dermatofibroma         & 197            \\
        Vascular lesion        & 63             \\
        Squamos cell carcinoma & 64             \\
        \bottomrule
    \end{tabular}
    \caption{Number of Samples for each class in ISIC-2019}
\end{table}
\paragraph{MIO-TCD} 11 classes, label distribution of the entire dataset is imbalanced.
\\
Class Distribution of entire dataset:
\begin{table}[]
    \begin{tabular}{ll}
    Class                 & Whole Dataset \\
    \midrule
    Articulated Truck     & 10346         \\
    Background            & 16000         \\
    Bicycle               & 2284          \\
    Bus                   & 10316         \\
    Car                   & 260518        \\
    Motorcycle            & 1982          \\
    Non-motorized vehicle & 1751          \\
    Pedestrian            & 6262          \\
    Pickup truck          & 50906         \\
    Single unit truck     & 5120          \\
    Work van              & 9679         
    \end{tabular}
    \caption{Number of samples for each class in MIO-TCD}
\end{table}

\subsection{Label Regimes}
Each label regime is defined by its starting budget and the corresponding acquisition size.
\begin{table}[]
\begin{tabular}{llll}
Label Regime & Starting Budget             & Query Size                  & Query Steps \\
Low          & 5xC   & 5xC   & 9           \\
Medium       & 25xC  & 25xC  & 9           \\
High         & 100xC & 100xC & 9           \\
Ultra-High   & 500xC & 500xC & (4-9           
\end{tabular}
\caption{The different label regimes we defined with their corresponding parameters. For CIFAR-100 they deviate due to the higher amount of classes w.r.t. the dataset size.}
\end{table}

\subsubsection{Label Regime in depth for imbalanced datasets}
\begin{table}[]
    \centering
    \begin{adjustbox}{width=.5\textwidth}
    \begin{tabular}{l|c|c|c|c|c}
         Regime& CIFAR-10 & CIFAR-100 & CIFAR-10 LT & Mio-TCD & ISIC-2019  \\
         \hline
         Low-Label& 50-500 & 500-5000 & 50-500 & 55-550 & 40-400 \\
         Medium-Label & 250-2500 & 1000-10000 & 250-2500 & 275 - 2750 & 200-2000 \\
         High-Label & 1000-10000 & 5000-25000 & 1000-10000 & 1100-11000 & 800-8000\\
         Ultra-High-Label & 5000-25000 & - & - & 5500-55000 & 4000-16000\\
    \end{tabular}
    \end{adjustbox}
    \caption{Label regimes on different datasets}
    \label{tab:label-regimes}
\end{table}
\section{Models}
Sweeped Hyper-Params are listed and final Hparams are listed
% Carsten Makes Models!
% Most information is in appendix -> Model Description: https://docs.google.com/document/d/1O5b6zTE07QMIIuMsvP2ET0MvFj6nLppfpOMmkTzPt-Q/edit#heading=h.iuu9am48258e
\paragraph{Model Architecture and Training}
% On each training step the model is trained from its initialization to avoid a `mode collapse'. 
% Further we selected the best checkpoint based on validation dataset performance.
As already mentioned a ResNet-18 \cite{heDeepResidualLearning2016} is the backbone for all of our experiments without weight decay on bias parameters as proposed by \cite{}. 
If not otherwise noted, a nesterov momentum optimizer with momentum $0.9$ is used.
For Self-SL models we use a two layer MLP as a classification head to make better use of the representations. 
To obtain bayesian models we add dropout on the final representations before the classification head with probability (P=0.5) following \cite{galDeepBayesianActive2017a}. 
Further for all experiments on imbalanced datasets we use weighted CE-Loss following \cite{munjalRobustReproducibleActive2022a} if not otherwise noted.
Models trained purely on the labeled dataset upsample it to a size of 5500 following \cite{kirschBatchBALDEfficientDiverse2019a}. 
\\
\textbf{ST} models were trained for 200 epochs with Cosine Annealing and 10 epochs warmup. \\
\textbf{Self-SL} pre-trained models were trained for 80 epochs with a reduction of the learning rate with a factor of 10 every 20 epochs.
The complete setup of the training for SimCLR is described in the appendix ... and the implementation is based on \cite{}\\
For both ST and Self-SL the HP sweep has 8 distinct settings sweeping: 2 data augmentations (Randaugment \cite{} or Standard transformations), 2 learning rate and 2 weight decay values.
\textbf{Semi-SL} model training is identical to the one proposed except that we do not use exponentially moving average models and restrict the training step from 1E6 to 2E5. The implementation used in our experiments is based on the open-source implementation and Kekmodel. We always selected the final model after training for all further steps.
On imbalanced datasets we changed the supervised term also the weighted CE-Loss and used distribution alignment on every dataset except for CIFAR-10 since it improved performance. 
The swept HPs for Semi-SL models are weight decay and learning rate. 
\subsection{Basic}
\subsubsection{Sweeped Hparams}
\subsubsection{Final Hparams per Dataset \& Performance}
\subsubsection{Ablation Classficatio Head MLP}
\subsection{Pre-Trained Finetuning}
\subsubsection{Hparams SimCLR}
\subsubsection{Sweeped Hparams}
\subsubsection{Final Hparams per Dataset \& Performance }
\subsection{FixMatch}
\subsubsection{Sweeped Hparams}
\subsubsection{Final Hparams per Dataset \& Performance}
\subsection{Self-SL + FixMatch}
\subsubsection{Sweeped Hparams}
\subsubsection{Final Hparams per Dataset \& Performance}
\section{RandAugment Parameters}
\section{Detailed Plots for single Experiments}
\subsection{CIFAR-10}
\begin{figure}
    \centering
    \includegraphics[width=\linewidth]{deep-active-plots/CIFAR-10/Accuracy/plot-full_train-basic_yshared-False_bound-False.pdf}
    \caption{CIFAR-10 Basic Models}
    \label{fig:app-cifar10-full-basic}
\end{figure}
\begin{figure}
    \centering
    \includegraphics[width=\linewidth]{deep-active-plots/CIFAR-10/Accuracy/plot-full_train-Self-SL_yshared-False_bound-False.pdf}
    \caption{CIFAR-10 Self-Supervised Pre-Trained Models}
    \label{fig:app-cifar10-full-SelfSL}
\end{figure}
\begin{figure}
    \centering
    \includegraphics[width=\linewidth]{deep-active-plots/CIFAR-10/Accuracy/plot-full_train-Sem-SL_yshared-False_bound-False.pdf}
    \caption{CIFAR-10 Semi-Supervised Pre-Trained Models}
    \label{fig:app-cifar10-full-SemSL}
\end{figure}

\subsection{CIFAR-100}
\begin{figure}
    \centering
    \includegraphics[width=\linewidth]{deep-active-plots/CIFAR-100/Accuracy/plot-full_train-basic_yshared-False_bound-False.pdf}
    \caption{CIFAR-100 Basic Models}
    \label{fig:app-cifar100-full-basic}
\end{figure}
\begin{figure}
    \centering
    \includegraphics[width=\linewidth]{deep-active-plots/CIFAR-100/Accuracy/plot-full_train-Self-SL_yshared-False_bound-False.pdf}
    \caption{CIFAR-100 Self-Supervised Pre-Trained Models}
    \label{fig:app-cifar100-full-SelfSL}
\end{figure}
\begin{figure}
    \centering
    \includegraphics[width=\linewidth]{deep-active-plots/CIFAR-100/Accuracy/plot-full_train-Sem-SL_yshared-False_bound-False.pdf}
    \caption{CIFAR-100 Semi-Supervised trained Models}
    \label{fig:app-cifar100-full-SemSL}
\end{figure}
\subsection{CIFAR-10 LT}
\begin{figure}
    \centering
    \includegraphics[width=\linewidth]{deep-active-plots/CIFAR-10-LT/Accuracy/plot-full_train-basic_yshared-False_bound-False.pdf}
    \caption{CIFAR-10 LT Basic Models}
    \label{fig:app-cifar10LT-full-basic}
\end{figure}
\begin{figure}
    \centering
    \includegraphics[width=\linewidth]{deep-active-plots/CIFAR-10-LT/Accuracy/plot-full_train-Self-SL_yshared-False_bound-False.pdf}
    \caption{CIFAR-10 LT Self-Supervised Pre-Trained Models}
    \label{fig:app-cifar10LT-full-SelfSL}
\end{figure}
\begin{figure}
    \centering
    \includegraphics[width=\linewidth]{deep-active-plots/CIFAR-10-LT/Accuracy/plot-full_train-Sem-SL_yshared-False_bound-False.pdf}
    \caption{CIFAR-10 LT Semi-Supervised Pre-Trained Models}
    \label{fig:app-cifar10LT-full-SemSL}
\end{figure}
\subsection{MIO-TCD}
\begin{figure}
    \centering
    \includegraphics[width=\linewidth]{deep-active-plots/MIO-TCD/Balanced-Accuracy/plot-full_train-basic_yshared-False_bound-False.pdf}
    \caption{MIO-TCD Basic Models}
    \label{fig:app-miotcd-full-basic}
\end{figure}
\begin{figure}
    \centering
    \includegraphics[width=\linewidth]{deep-active-plots/MIO-TCD/Balanced-Accuracy/plot-full_train-Self-SL_yshared-False_bound-False.pdf}
    \caption{MIO-TCD Self-Supervised Pre-Trained Models}
    \label{fig:app-miotcd-full-SelfSL}
\end{figure}
% \begin{figure}
%     \centering
%     \includegraphics[width=\linewidth]{deep-active-plots/CIFAR-10-LT/Accuracy/plot-full_train-Sem-SL_yshared-False_bound-False.pdf}
%     \caption{MIO-TCD Semi-Supervised Pre-Trained Models}
%     \label{fig:app-miotcd-full-SemSL}
% \end{figure}

\subsection{ISIC-2019}
\begin{figure}
    \centering
    \includegraphics[width=\linewidth]{deep-active-plots/ISIC-2019/Balanced-Accuracy/plot-full_train-basic_yshared-False_bound-False.pdf}
    \caption{ISIC-2019 Basic Models}
    \label{fig:app-isci2019-full-basic}
\end{figure}
\begin{figure}
    \centering
    \includegraphics[width=\linewidth]{deep-active-plots/ISIC-2019/Balanced-Accuracy/plot-full_train-Self-SL_yshared-False_bound-False.pdf}
    \caption{ISIC-2019 Self-Supervised Pre-Trained Models}
    \label{fig:app-isci2019-full-SelfSL}
\end{figure}
% \begin{figure}
%     \centering
%     \includegraphics[width=\linewidth]{deep-active-plots/CIFAR-10-LT/Accuracy/plot-full_train-Sem-SL_yshared-False_bound-False.pdf}
%     \caption{ISIC-2019 Semi-Supervised Pre-Trained Models}
%     \label{fig:app-miotcd-full-SemSL}
% \end{figure}
\section{}

\section{Batch Entropy}
\section{Dataset Entropy}
\section{Performance Comparison across Papers}
\subsection{CIFAR-10}
\begin{table*}[]
    \centering
    \begin{tabular}{llllllll}
\multicolumn{4}{l}{Information}                         & \multicolumn{4}{l}{Number Labeled Training Samples} \\
Paper           & Method  & Model       & Source        & 5k          & 10k         & 15k        & 20k        \\
QBC             & SL      & DenseNet121 & Munjal et al. & 74          & 82,5        &            &            \\
VAAL            & SL      & VGG16       & Munjal et al. & 61,35       & 68,17       & 72,96      & 75,99      \\
CoreSet         & SL      & VGG16       & Munjal et al. & 60          & 68          & 71         & 74         \\
Munjal-SR       & SL      & VGG16       & Munjal et al. & 82,16       & 85,07       & 89,43      & 91,16      \\
LLAL            & SL      & ResNet18    & Munjal et al. & 81          & 87          & -          & -          \\
CoreCGN         & SL      & ResNet18    & Munjal et al. & 80          & 85,5        & -          & -          \\
TA-VAAL         & SL      & ResNet18    & Munjal et al. & 81          & 87,5        & -          & -          \\
Munjal-SR       & SL      & ResNet18    & Munjal et al. & 84,69       & 88,45       & 89,98      & 92,29      \\
Mittal et al.   & SL      & WRN28-2     & Graph         & 82,5        & 86          & 90,7       & 92         \\
Mittal et al.   & Semi-SL & WRN28-2     & Graph         & 92,5        & 93,8        & 94         & 94,5       \\
Bengar et al.   & SL      & ResNet18    & Graph         & 73          & 81          & 85         & 88         \\
Bengar et al.   & Self-SL & ResNet18    & Graph         & 89,5        & 90,5.       & 91         & 91,5       \\
Yi et al.       & SL      & ResNet18    & Graph         & 78          & 86          & -          & -          \\
Krishnan et al. & SL      & ResNet18    & Graph         & 78          & 86          & -          & -          \\
Ours            & SL      & ResNet18    & Table         & 85,50       & 90,50       & -          & -          \\
Ours            & Self-SL & ResNet18    & Table         & 90,05       & 91,40       & -          & -         
\end{tabular}

    \caption{Results on the high label regime for CIFAR-10}
    \label{tab:app-random-cifar10-high}
\end{table*}
\begin{table*}[]
    \centering
    \begin{tabular}{llllllll}
\multicolumn{4}{l}{Information}               & \multicolumn{4}{l}{Number Labeled Training Samples} \\
Paper           & Method  & Model    & Source & 250         & 500         & 1000       & 2000       \\
Mittal et al.   & SL      & WRN28-2  & Graph  & 36          & 48          & 57         & 73         \\
Mittal et al.   & Semi-SL & WRN28-2  & Graph  & 82          & 85          & 88         & 91         \\
Bengar et al.   & SL      & ResNet18 & Graph  & -           & 38          & 45         & 55         \\
Bengar et al.   & Self-SL & ResNet18 & Graph  & 83          & 85          & 87         & 88         \\
Yi et al.       & SL      & ResNet18 & Graph  & -           & -           & 47,5       & 56         \\
Krishnan et al. & SL      & ResNet18 & Graph  & -           & -           & 47         & 60         \\
Gao et al.      & Semi-SL & WRN28-2  & Graph  & 90,23       & -           & 92,5       & 92,5       \\
Ours            & SL      & ResNet18 & Table  & 46,95       & 61,15       & 72,38      & 79,83      \\
Ours            & Self-SL & ResNet18 & Table  & 81,41       & 84,13       & 86,22      & 88,26      \\
Ours            & Semi-SL & ResNet18 & Graph  & 93          & 94          & 94,5       & 95        
\end{tabular}
    \caption{Results on the medium label regime for CIFAR-10}
    \label{tab:app-random-cifar10-med}
\end{table*}
\begin{table*}[]
    \centering
    \begin{tabular}{lllllll}
\multicolumn{4}{l}{Information}             & \multicolumn{3}{l}{Number Labeled Training Samples} \\
Paper         & Method  & Model    & Source & 50              & 100             & 200             \\
Bengar et al. & Self-SL & ResNet18 & Graph  & 62              & 77              & 81              \\
Gao et al.    & Semi-SL & WRN28-2  & Table  & -               & 47,85           & 89,20           \\
Ours          & SL      & ResNet18 & Table  & 25,14           & 32,33           & 44,36           \\
Ours          & Self-SL & ResNet18 & Table  & 71,31           & 76,80           & 81,18           \\
Ours          & Semi-SL & ResNet18 & Graph  & 90              & 91              & 93             
\end{tabular}
    \caption{Results on the low label regime for CIFAR-10}
    \label{tab:app-random-cifar10-low}
\end{table*}
\subsection{CIFFAR-100}
\begin{table*}[]
    \centering
    \begin{tabular}{llllllll}
\multicolumn{4}{l}{Information}             & \multicolumn{4}{l}{Number Labeled Training Samples} \\
Paper         & Method  & Model    & Source & 5k          & 10k         & 15k        & 20k        \\
Munjal et al. & SL      & VGG16    & Graph  & 39,44       & 49          & 55         & 59         \\
Munjal et al. & SL      & ResNet18 & Table  & ?           & 61,06       & 66,92      & 69,83      \\
Mittal et al. & SL      & WRN28-2  & Graph  & 44,9        & 58          & 64         & 68         \\
Mittal et al. & Semi-SL & WRN28-2  & Graph  & 59          & 65          & 70         & 71         \\
Bengar et al. & SL      & ResNet18 & Graph  & 27          & 45          & 52         & 58         \\
Bengar et al. & Self-SL & ResNet18 & Table  & 60          & 63          & 63,5       & 64         \\
Gao et al.    & Semi-SL & WRN28-2  & Table  & 63,35       & 67          & 68         & 70         \\
Ours          & SL      & ResNet18 & Table  & 49,16       & 61,25       & 66,72      & 70,25      \\
Ours          & Self-SL & ResNet18 & Table  & 60,36       & 64,77       & 68,37      & 70,71     
\end{tabular}
    \caption{Results on the high label regime for CIFAR-100}
    \label{tab:app-random-cifar100-high}
\end{table*}
\begin{table*}[]
    \centering
    \begin{tabular}{llllllll}
\multicolumn{4}{l}{Information}             & \multicolumn{4}{l}{Number Labeled Training Samples} \\
Paper         & Method  & Model    & Source & 500         & 1000        & 2000       & 2500       \\
Mittal et al. & SL      & WRN28-2  & Graph  & 9           & 12          & 24         & 34         \\
Mittal et al. & Semi-SL & WRN28-2  & Graph  & 26          & 35,5        & 44,5       & 49         \\
Bengar et al. & SL      & ResNet18 & Graph  & 9           & 12          & 17         & -          \\
Bengar et al. & Self-SL & ResNet18 & Table  & 47          & 50          & 56         & -          \\
Ours          & SL      & ResNet18 & Table  & 14,03       & 22,39       & 31,99      & 36,27      \\
Ours          & Self-SL & ResNet18 & Table  & 37,32       & 45,22       & 52,16      & 54,71      \\
Ours          & Semi-SL & ResNet18 & Graph  & 37,5        & -           & 54,5       & -         
\end{tabular}
    \caption{Results on the medium label regime for CIFAR-100}
    \label{tab:app-random-cifar100-med}
\end{table*}
