# Supplementary material for: Navigating the Pitfalls of Active Learning Evaluation: A Systematic Framework for Meaningful Performance Assessment
Source: arXiv:2301.10625 source file (2023-11-03)
Supplement: Supplementary file 3 [file 05_results_old.tex]

\section{Results, in more detail}\label{app:results}
\subsection{Main results}
\textbf{General observations:}
% \paragraph{General Observations}
For all datasets, the overall performance of models was primarily determined by the training strategy and the HP selection, with the benefits of AL being generally smaller compared to the proper selection of both.
For the three toy datasets Semi-SL generally performed best, followed by Self-SL and ST last, whereas for the two real-world datasets Semi-SL showed no substantial improvement over ST in the first training stage, and therefore further runs were omitted.
Also, the performance gains for Self-SL models with AL are generally smaller compared to ST models. 
For Semi-SL there were generally only very small performance gains or substantially worse performance with AL observed.
Concerning the effect of AL, the high-label regime proved to work for ST models on all datasets and Self-SL models.
On the two real-world datasets, MIO-TCD and ISIC-2019 a dip in performance at ~7k samples for all ST models could be observed. 
This behavior is ablated in \cref{app_s:hparams-imbalance}.
\subsubsection{CIFAR-10}
\begin{figure}
    \centering
    % \includegraphics[width=\linewidth]{deep-active-plots/CIFAR-10/Accuracy/plot-full_train-basic_yshared-False_bound-False.pdf}
    \includegraphics[width=\linewidth]{appendix_final_plots/CIFAR-10/full/standard/accuracy/sharey-false_upper_bound-false.png}
    \caption{CIFAR-10 ST}
    \label{fig:app-cifar10-full-basic}
\end{figure}
\paragraph{ST} 
Results are shown in \cref{fig:app-cifar10-full-basic}.

\begin{itemize}
    \item Low-label regime: BALD and Core-Set perform on the same level as random. Entropy performs worse than random, presumably due to cold-start.
    \item Medium-label regime: BALD and Core-Set perform on the same level as random. Entropy performs worse in the beginning but catches up with random in the end.
    \item High-label regime: Core-Set outperforms random from 3k samples onward, BALD from 6k samples onward and Entropy performs worse in the beginning but catches up later. All QMs outperform random at 10k samples with similar performance.
\end{itemize}

\begin{figure}
    \centering
    % \includegraphics[width=\linewidth]{deep-active-plots/CIFAR-10/Accuracy/plot-full_train-Self-SL_yshared-False_bound-False.pdf}
    \includegraphics[width=\linewidth]{appendix_final_plots/CIFAR-10/full/self-sl/accuracy/sharey-false_upper_bound-false.png}
    \caption{CIFAR-10 Self-SL }
    \label{fig:app-cifar10-full-SelfSL}
\end{figure}
\paragraph{Self-SL}
Results are shown in \cref{fig:app-cifar10-full-SelfSL}.
\begin{itemize}
    \item Low-label regime: Core-Set outperforms random over from the beginning, BALD starts worse than random but catches up with more queries at 250 samples and Entropy also performs worse but catches up at 400 samples.
    \item Medium-label regime: All QMs perform very similarly to random with none substantially outperforming or underperforming.
    \item High-label regime: BALD outperforms is best performing QM outperforming random on all points. Entropy is second best followed by Core-Set, all outperforming random queries
\end{itemize}

\begin{figure}
    \centering
    % \includegraphics[width=\linewidth]{deep-active-plots/CIFAR-10/Accuracy/plot-full_train-Sem-SL_yshared-False_bound-False.pdf}
    \includegraphics[width=\linewidth]{appendix_final_plots/CIFAR-10/full/sem-sl/accuracy/sharey-false_upper_bound-false.png}
    \caption{CIFAR-10 Semi-SL}
    \label{fig:app-cifar10-full-SemSL}
\end{figure}

\paragraph{Semi-SL}
Results are shown in \cref{fig:app-cifar10-full-SemSL}.

\begin{itemize}
    \item Low-label regime: noise is very high but Entropy leads to a strong reduction in performance at 100 samples compared to random.
    \item Medium-label regime: Entropy indicates a small performance increase over random samples. Core-Set underperforms random queries.
\end{itemize}


\subsubsection{CIFAR-100}
\begin{figure}
    \centering
    % \includegraphics[width=\linewidth]{deep-active-plots/CIFAR-100/Accuracy/plot-full_train-basic_yshared-False_bound-False.pdf}
    \includegraphics[width=\linewidth]{appendix_final_plots/CIFAR-100/full/standard/accuracy/sharey-false_upper_bound-false.png}
    \caption{CIFAR-100 ST}
    \label{fig:app-cifar100-full-basic}
\end{figure}
\paragraph{ST}
Results are shown in \cref{fig:app-cifar100-full-basic}.

\begin{itemize}
    \item Low-label regime: BALD performs similarly to random, Core-Set performs a little bit worse than random and Entropy performs substantially worse than random with a decreasing trend.
    \item Medium-label regime: BALD performs identically to random and might improve from 8k samples onward. Core-Set performs similarly as random. Entropy starts performing worse but closes the performance gap till the end.
    \item High-label regime: All QMs outperform random. BALD performs best on all stages, Core-Set is better than random on all stages but Entropy has a higher final performance.
\end{itemize}

\begin{figure}
    \centering
    % \includegraphics[width=\linewidth]{deep-active-plots/CIFAR-100/Accuracy/plot-full_train-Self-SL_yshared-False_bound-False.pdf}
    \includegraphics[width=\linewidth]{appendix_final_plots/CIFAR-100/full/self-sl/accuracy/sharey-false_upper_bound-false.png}
    \caption{CIFAR-100 Self-SL }
    \label{fig:app-cifar100-full-SelfSL}
\end{figure}
\paragraph{Self-SL}
Results are shown in \cref{fig:app-cifar100-full-SelfSL}.

\begin{itemize}
    \item Low-label regime: No QM performs as well as random. Core-Set performs closest but falls off later, Entropy performs also worse and BALD performs worst.
    \item Medium-label regime: No QM performs as well as random. Core-Set performs closest but falls off later, Entropy performs also worse and BALD performs worst.
    \item High-label regime: All QMs outperform random. Entropy performs best and BALD and Core-Set perform similarly to each other.
\end{itemize}

\begin{figure} 
    \centering
    % \includegraphics[width=\linewidth]{deep-active-plots/CIFAR-100/Accuracy/plot-full_train-Sem-SL_yshared-False_bound-False.pdf}
    \includegraphics[width=\linewidth]{appendix_final_plots/CIFAR-100/full/sem-sl/accuracy/sharey-false_upper_bound-false.png}
    \caption{CIFAR-100 Semi-SL}
    \label{fig:app-cifar100-full-SemSL}
\end{figure}
\paragraph{Semi-SL}
Results are shown in \cref{fig:app-cifar100-full-SemSL}.

\begin{itemize}
    \item Low-label regime: random outperforms all QMs. Core-Set is second best and Entropy performs worst.
    \item Medium-label regime: random outperforms all QMs. Entropy has a similar final accuracy to random.
\end{itemize}

\subsubsection{CIFAR-10 LT}
\begin{figure}
    \centering
    % \includegraphics[width=\linewidth]{deep-active-plots/CIFAR-10-LT/Accuracy/plot-full_train-basic_yshared-False_bound-False.pdf}
    \includegraphics[width=\linewidth]{appendix_final_plots/CIFAR-10-LT/full/standard/accuracy/sharey-false_upper_bound-false.png}
    \caption{CIFAR-10 LT ST}
    \label{fig:app-cifar10LT-full-basic}
\end{figure}

\paragraph{ST}
Results are shown in \cref{fig:app-cifar10LT-full-basic}.

\begin{itemize}
    \item Low-label regime: BALD and Core-Set outperform random and lead to substantial 6-8\% benefit in accuracy. Entropy performs slightly worse than random.
    \item Medium-label regime: Core-Set performs best leading to a 10-12\% increase in accuracy at 2k samples followed by BALD also substantially improving over random and Entropy performs a little bit worse than random.
    \item High-label regime: Core-Set performs best leading to more stable performance across all stages. Entropy performance is generally worse than random but catches up at 10k samples and BALD performs much worse than random. Note: slight dip in performance for 3k samples (high-label) with all QMs except for Core-Set. This is ablated in \cref{app_s:hparams-imbalance} and might be due to handling imbalanced datasets with weighted CE-Loss.
\end{itemize}


\begin{figure}
    \centering
    % \includegraphics[width=\linewidth]{deep-active-plots/CIFAR-10-LT/Accuracy/plot-full_train-Self-SL_yshared-False_bound-False.pdf}
    \includegraphics[width=\linewidth]{appendix_final_plots/CIFAR-10-LT/full/self-sl/accuracy/sharey-false_upper_bound-false.png}
    \caption{CIFAR-10 LT Self-SL }
    \label{fig:app-cifar10LT-full-SelfSL}
\end{figure}
\paragraph{Self-SL}
Results are shown in \cref{fig:app-cifar10LT-full-SelfSL}.

\begin{itemize}
    \item Low-label regime: BALD is best performing leading to 4\% accuracy gain over random at 500 samples. Entropy is also outperforming random while Core-Set performs a little bit worse than random.
    \item Medium-label regime: All QMs outperform random with BALD and Entropy best performing (Entropy has lower variance) and Core-Set still outperforms random but is substantially worse than uncertainty-based QMs.
    \item High-label regime: All QMs outperform random with BALD and Entropy best performing (Entropy has lower variance) and Core-Set still outperforms random but is substantially worse than uncertainty-based QMs while catching up at later stages.
\end{itemize}

\begin{figure}
    \centering
    % \includegraphics[width=\linewidth]{deep-active-plots/CIFAR-10-LT/Accuracy/plot-full_train-Sem-SL_yshared-False_bound-False.pdf}
    \includegraphics[width=\linewidth]{appendix_final_plots/CIFAR-10-LT/full/sem-sl/accuracy/sharey-false_upper_bound-false.png}
    \caption{CIFAR-10 LT Semi-SL}
    \label{fig:app-cifar10LT-full-SemSL}
\end{figure}
\paragraph{Semi-SL}
Results are shown in \cref{fig:app-cifar10LT-full-SemSL}.

\begin{itemize}
    \item Low-label regime: Trend is unclear everything within variances but Core-Set might lead to benefits.
    \item Medium-label regime: Core-Set substantially improves performance over random and Entropy. Note: Training of Semi-SL methods might have been prone to lower accuracies on imbalanced datasets.
\end{itemize}

\subsubsection{MIO-TCD}
\begin{figure}
    \centering
    % \includegraphics[width=\linewidth]{deep-active-plots/MIO-TCD/Balanced-Accuracy/plot-full_train-basic_yshared-False_bound-False.pdf}
    \includegraphics[width=\linewidth]{appendix_final_plots/MIO-TCD/full/standard/balanced-accuracy/sharey-false_upper_bound-false.png}
    \caption{MIO-TCD ST}
    \label{fig:app-miotcd-full-basic}
\end{figure}
\paragraph{ST}
Results are shown in \cref{fig:app-miotcd-full-basic}.

\begin{itemize}
    \item Low-label regime: Core-Set is only QM outperforming random. Entropy and BALD perform a slightly worse than random.
    \item Medium-label regime: Core-Set is the best performing QM substantially outperforming random, closely followed by BALD. Entropy performs much worse than random QM.
    \item High-label regime: Core-Set is the best performing QM outperforming random. BALD shows extremely high variance but generally also outperforms random (mean) and Entropy performs substantially worse than random even decreasing the absolute performance. Note: Dip in performance for the high-label regime at approximately 7k samples is ablated in \cref{app_s:hparams-imbalance}.
\end{itemize}

\begin{figure}
    \centering
    % \includegraphics[width=\linewidth]{deep-active-plots/MIO-TCD/Balanced-Accuracy/plot-full_train-Self-SL_yshared-False_bound-False.pdf}
    \includegraphics[width=\linewidth]{appendix_final_plots/MIO-TCD/full/self-sl/balanced-accuracy/sharey-false_upper_bound-false.png}
    \caption{MIO-TCD Self-SL }
    \label{fig:app-miotcd-full-SelfSL}
\end{figure}
\paragraph{Self-SL}
Results are shown in \cref{fig:app-miotcd-full-SelfSL}.

\begin{itemize}
    \item Low-label regime: Core-Set is best performing and Entropy second best, both perform similarly to random. BALD performs much worse than random queries.
    \item Medium-label regime: Entropy performs a little bit worse than random. Core-Set performs slightly worse than Entropy and BALD performs substantially worse.
    \item High-label regime: Core-Set and Entropy perform similarly to random. BALD decreases absolute performance in the first query step and performs substantially worse than random.
\end{itemize}

\paragraph{Semi-SL}
% Results are shown in \cref{fig:app-cifar10-full-SemSL}.\\
We performed no AL experiments due to the bad performance of Semi-SL on the starting budgets.
More information can be found in \cref{app_s:semi-sl}.

\subsubsection{ISIC-2019}
\begin{figure}
    \centering
    % \includegraphics[width=\linewidth]{deep-active-plots/ISIC-2019/Balanced-Accuracy/plot-full_train-basic_yshared-False_bound-False.pdf}
    \includegraphics[width=\linewidth]{appendix_final_plots/ISIC-2019/full/standard/balanced-accuracy/sharey-false_upper_bound-false.png}
    \caption{ISIC-2019 ST}
    \label{fig:app-isci2019-full-basic}
\end{figure}
\paragraph{ST}
Results are shown in \cref{fig:app-isci2019-full-basic}.

\begin{itemize}
    \item Low-label regime: All QMs perform on the same level as random with Core-Set maybe giving a minor benefit. The variance is very high. 
    \item Medium-label regime: Core-Set leads to substantial benefit over random queries. BALD and Entropy start with similar performance but lead to reduced performance even reducing absolute performance from approx. 1k samples onward.
    \item High-label regime: Core-Set is the best performing QM giving substantial gain over random while Entropy performs similarly to random. BALD performs worse than random from 4k samples onward even reducing absolute performance. Note: The dip in performance for the high-label regime at approximately 7k samples is ablated in \cref{app_s:hparams-imbalance}.
\end{itemize}

\begin{figure}
    \centering
    % \includegraphics[width=\linewidth]{deep-active-plots/ISIC-2019/Balanced-Accuracy/plot-full_train-Self-SL_yshared-False_bound-False.pdf}
    \includegraphics[width=\linewidth]{appendix_final_plots/ISIC-2019/full/self-sl/balanced-accuracy/sharey-false_upper_bound-false.png}
    \caption{ISIC-2019 Self-SL Pre-Trained Models}
    \label{fig:app-isci2019-full-SelfSL}
\end{figure}
\paragraph{Self-SL}
Results are shown in \cref{fig:app-isci2019-full-SelfSL}.

\begin{itemize}
    \item Low-label regime: BALD outperforms random while Entropy performs a little bit worse than random and Core-Set is the worst performing.
    \item Medium-label regime: BALD is the best performing QM. Entropy performs slightly better than random and Core-Set performs as well as random.
    \item High-label regime: Entropy is best performing QM. Core-Set performs a little bit better than random and BALD initially performs better than random but then performs worse than random.
\end{itemize}


\paragraph{Semi-SL}
We performed no AL experiments due to the bad performance of Semi-SL on the starting budgets.
More information can be found in \cref{app_s:semi-sl}.
% Results are shown in \cref{fig:app-cifar10-full-SemSL}.\\
% Results showing the performance of the wideresnet28-10 on CIFAR100 with the standard FixMatch training using our implementation are shown in table \cref{}.

\subsection{Low-Label Query Size}\label{app_s:low-qs}
% \input{appendix/tables/QS-CIFAR_0}
% \input{appendix/tables/QS-CIFAR_1}
% \input{appendix/tables/QS-ISIC_0}
% \input{appendix/tables/QS-ISIC_1}



% \subsection{Low-Label Cold-Start Ablation}
% The results for CIFAR-100 using a smaller acquisition size and MIO-TCD using a downsampled pool are here set into context in \cref{fig:app-bb-exp} than in \cref{sec:discussion}.
% Here would like to highlight that BALD substantially benefits from smaller query sizes on CIFAR-100.
% Further, on MIO-TCD the smaller pool leads to a substantial benefit for BALD and BatchBALD brings even greater improvements.
% This shows similarities to the behavior \cite{kirschBatchBALDEfficientDiverse2019a} observe on Repeated MNIST for BALD and BatchBALD.
% Based on this, we hypothesize that MIO-TCD has more samples with strong similarities to each other that the greedy QMs select for annotation and therefore lose performance compared to random queries.
% \begin{figure}
%     \centering
%     % \includegraphics{}
%         \begin{subfigure}[b]{0.4\linewidth}
%         \centering
%         % \includegraphics[width=\linewidth]{deep-active-plots/CIFAR-100/Accuracy/plot-low-bb_train-Self-SL_yshared-False_bound-False.pdf}
%         \includegraphics[width=\linewidth]{appendix_final_plots/CIFAR-100/bb/self-sl/accuracy/sharey-false_upper_bound-false.png}
%         \caption{CIFAR-100 with query size reduced from 500 to 50.}
%         \label{fig:cifar100-bb}
%     \end{subfigure}
%     \begin{subfigure}[b]{0.59\linewidth}
%         \centering
%         % \includegraphics[width=\linewidth]{deep-active-plots/MIO-TCD/Balanced-Accuracy/plot-low-bb-fulll_train-Self-SL_yshared-True_bound-False.pdf}
%         \includegraphics[width=\linewidth]{appendix/plots/MIO-TCD/Low-Label-Addition/plot-low-bb-fulll_train-Self-SL_yshared-True_bound-False.png}
%         \caption{MIO-TCD with Pool downsampled from 300k to 50k.}
%         \label{fig:mio-tcd-bb}
%     \end{subfigure}
%     \caption{Detailed results for the low-label cold-start ablation on CIFAR-100 and MIO-TCD. On CIFAR-100 low-label regime with a query size of 500 for 1k samples, the accuracy of BALD is approx. 42\%.
%     }
%     \label{fig:app-bb-exp}
% \end{figure}


\subsection{Semi-Supervised Learning}\label{app_s:semi-sl}
Results of FixMatch for all HPs on the whole validation splits are shown separately for MIO-TCD in \cref{tab:miotcd-semsl} and ISIC-2019 in \cref{tab:isic2019-semsl}.
Based on the performance which did not improve substantially over even ST models we decided to omit all further AL experiments.

\begin{table}[]
    \centering
    \begin{adjustbox}{width=\linewidth}
    \input{appendix/tables/ISIC-2019-Semi-SL}
    \end{adjustbox}
    \caption{ISIC-2019 FixMatch results reported on the three whole validation splits (balanced accuracy in \%).
    Compared to ST with 28\%  and Self-SL 33\% balanced accuracy on the test split with 40 labeled train samples.}
    \label{tab:isic2019-semsl}
\end{table}

\begin{table}[]
    \centering
    \begin{adjustbox}{width=\linewidth}
    \input{appendix/tables/MIO-TCD-Semi-SL}
    \end{adjustbox}
    \caption{MIO-TCD FixMatch results reported on the three whole validation splits (balanced accuracy in \%).
    Compared to ST with 28\% and Self-SL with 42\% balanced accuracy on the test split with 55 labeled train samples.}
    \label{tab:miotcd-semsl}
\end{table}
